# Supplementary material for: Compound-tunable embedding potential method to model local electronic excitations on $f$-element ions in solids: Pilot relativistic coupled cluster study of Ce and Th impurities in yttrium orthophosphate, YPO$_4$
Source: arXiv:2310.09240 source file (2024-02-15)
Supplement: Supplementary file 1 [file supplementary.pdf]

# Supporting information: Compound-tunable embedding potential method to model local electronic excitations on $f$-element ions in solids: Pilot relativistic coupled cluster study of Ce and Th impurities in yttrium orthophosphate, $YPO_4$

A. V. Oleynichenko,[1,2,*] Y. V. Lomachuk,[1,†] D. A. Maltsev,[1]
N. S. Mosyagin,[1] V. M. Shakhova,[1] A. Zaitsevskii,[1,3] and A. V. Titov[1,4,‡]

[1]*B. P. Konstantinov Petersburg Nuclear Physics Institute of National Research Center "Kurchatov Institute" (NRC "Kurchatov Institute" – PNPI), Gatchina, Leningrad district 188300, Russia*
[2]*Moscow Institute of Physics and Technologies (National Research University), Institutskij pereulok 9, Dolgoprudny Moscow region 141700, Russia*
[3]*Department of Chemistry, M. V. Lomonosov Moscow State University, Leninskie Gory 1/3, Moscow 119991, Russia*
[4]*Saint Petersburg State University, 7/9 Universitetskaya nab., 199034 St. Petersburg, Russia*

(Dated: January 14, 2024)

## CONTENTS

I. Introductory notes 1

II. Cluster models 2
A. $Y(PO_4)_6$@CTEP (big cluster) 2
B. $YO_8$@CTEP (minimal cluster) 6
C. $Ce(PO_4)_6$@CTEP (big cluster) 8
D. $CeO_8$@CTEP (minimal cluster) 11
E. $Th(PO_4)_6$@CTEP (big cluster) 13
F. $ThO_8$@CTEP (minimal cluster) 16

III. Pseudopotentials and basis sets the for main cluster 18
A. RPP and basis sets for DFT calculations 18
B. RPP and basis set for cerium (FS-RCC calculations) 24
C. RPP and basis set for thorium (FS-RCC calculations) 27

## I. INTRODUCTORY NOTES

Supporting information contains geometry parameters of all the cluster models constructed and discussed in the paper as well as pseudopotentials and basis sets used in relativistic coupled cluster calculations of excitation energies.

Cluster model obtained within the CTEP approach consists of:

- Cartesian coordinates of all main-cluster atoms, pseudoatoms of nearest cation (NCE) and anion (NAE) environment layers and additional fractional point charges placed at these pseudoatoms;
- Basis sets and relativistic pseudopotentials for the main-cluster atoms;
- Auxuliary basis sets and compound-tunable pseudopotentials (CTPPs) for pseudoatoms of NCE and NAE layers. CTPPs were parametrized according to Eq. (2) of the original article.

For basis sets and pseudopotentials the NWChem-like format is assumed.

* oleynichenko_av@pnpi.nrcki.ru
† lomachuk_yv@pnpi.nrcki.ru
‡ titov_av@pnpi.nrcki.ru

## II. CLUSTER MODELS

### A. $Y(PO_4)_6$@CTEP (big cluster)

```
# (atomic units)
#     charge         x              y              z

# main cluster

Y     0.0000    -0.00000000    -3.27709581     1.43262505
P     0.0000    -0.00000009    -9.83185559     4.29866088
P     0.0000     0.00000019    -3.27709542     7.16323167
P     0.0000    -0.00000012     3.27766418     4.29866046
P     0.0000     0.00000002    -3.27709487    -4.29798154
P     0.0000    -6.55475978    -3.27709521    -1.43341051
P     0.0000     6.55475965    -3.27709541    -1.43341060
O     0.0000    -0.00000056    -7.54078750     2.42661174
O     0.0000    -2.28900935    -3.27709779     5.28784020
O     0.0000    -0.00000044     0.98659171     2.42661625
O     0.0000    -0.00000092    -0.98808600    -2.42258964
O     0.0000    -0.00000064    -5.56610484    -2.42259086
O     0.0000    -4.26369047    -3.27709837     0.43863701
O     0.0000     4.26368934    -3.27709797     0.43863596
O     0.0000     2.28900936    -3.27709770     5.28784025
O     0.0000     0.00000051   -12.1171674      2.41881690
O     0.0000    -2.28807725    -9.83497502     6.17470878
O     0.0000     2.28807756    -9.83497451     6.17470887
O     0.0000     0.00000036    -0.98888644     9.03977640
O     0.0000     0.00000055    -5.56530043     9.03978212
O     0.0000    -0.00000045     5.56297249     2.41881132
O     0.0000    -2.28807801     3.28078884     6.17470869
O     0.0000     2.28807799     3.28078893     6.17470838
O     0.0000    -2.28820613    -3.27709279    -6.17452954
O     0.0000     2.28820770    -3.27709272    -6.17452868
O     0.0000    -6.55787953    -5.56517089    -3.30946148
O     0.0000    -6.55788091    -0.98901566    -3.30945569
O     0.0000    -8.84007092    -3.27709974     0.44643493
O     0.0000     6.55788161    -5.56517158    -3.30946090
O     0.0000     6.55788250    -0.98901601    -3.30945591
O     0.0000     8.84006947    -3.27709890     0.44643634

# nearest cation environment

Y     2.8312    -0.00000000    -9.83128744    -1.43262505
Y     2.8312    -6.55419162    -3.27709581     4.29787515
Y     2.8312    -0.00000000     3.27709581    -1.43262505
Y     2.8312     6.55419162    -3.27709581     4.29787515
Y     2.4478    -0.00000000   -16.38547907     1.43262505
Y     2.5681    -6.55419162    -9.83128744     7.16312525
Y     2.6649    -0.00000000    -9.83128744    10.02837535
Y     2.5681     6.55419162    -9.83128744     7.16312525
Y     2.5722    -0.00000000    -3.27709581    12.89362546
Y     2.6649    -0.00000000     3.27709581    10.02837535
Y     2.4478    -0.00000000     9.83128744     1.43262505
Y     2.5681    -6.55419162     3.27709581     7.16312525
Y     2.5681     6.55419162     3.27709581     7.16312525
Y     2.6649    -6.55419162    -3.27709581    -7.16312525
Y     2.5722    -0.00000000    -3.27709581   -10.02837535
```

```
Y     2.6649     6.55419162    -3.27709581    -7.16312525
Y     2.5681    -6.55419162    -9.83128744    -4.29787515
Y     2.5681    -6.55419162     3.27709581    -4.29787515
Y     2.4478   -13.10838325    -3.27709581     1.43262505
Y     2.5681     6.55419162    -9.83128744    -4.29787515
Y     2.5681     6.55419162     3.27709581    -4.29787515
Y     2.4478    13.10838325    -3.27709581     1.43262505

# additional fractional charges (simulating NAE)

q    -0.8609    -2.28797108    -9.83128744    -5.28676952
q    -0.7579     0.00000000   -14.09750798    -2.42151942
q    -0.6792     4.26622054    -9.83128744    -0.44373067
q    -0.6792    -4.26622054    -9.83128744    -0.44373067
q    -0.8609     2.28797108    -9.83128744    -5.28676952
q    -0.8609    -6.55419162    -5.56506690     8.15201963
q    -0.8609    -6.55419162    -0.98912472     8.15201963
q    -0.6792    -6.55419162    -7.54331635     3.30898077
q    -0.7579   -10.82041217    -3.27709581     5.28676952
q    -0.6792    -6.55419162     0.98912472     3.30898077
q    -0.8609    -2.28797108     3.27709581    -5.28676952
q    -0.6792     4.26622054     3.27709581    -0.44373067
q    -0.6792    -4.26622054     3.27709581    -0.44373067
q    -0.8609     2.28797108     3.27709581    -5.28676952
q    -0.7579    -0.00000000     7.54331635    -2.42151942
q    -0.8609     6.55419162    -5.56506690     8.15201963
q    -0.8609     6.55419162    -0.98912472     8.15201963
q    -0.6792     6.55419162    -7.54331635     3.30898077
q    -0.7579    10.82041217    -3.27709581     5.28676952
q    -0.6792     6.55419162     0.98912472     3.30898077
q    -0.1918     0.00000000   -20.65169961     2.42151942
q    -0.1553    -2.28797108   -16.38547907     5.28676952
q    -0.2635    -0.00000000   -18.67345015    -2.42151942
q    -0.4268    -4.26622054   -16.38547907     0.44373067
q    -0.4268     4.26622054   -16.38547907     0.44373067
q    -0.1553     2.28797108   -16.38547907     5.28676952
q    -0.5823    -6.55419162   -14.09750798     8.15201963
q    -0.0006    -8.84216271    -9.83128744    11.01726973
q    -0.4226    -6.55419162   -12.11925852     3.30898077
q    -0.0251   -10.82041217    -9.83128744     6.17423088
q    -0.5681    -4.26622054    -9.83128744    11.01726973
q    -0.1627     0.00000000   -12.11925852    13.88251983
q    -0.8339     0.00000000    -7.54331635    13.88251983
q    -0.5349     0.00000000   -14.09750798     9.03948098
q    -0.5681     4.26622054    -9.83128744    11.01726973
q    -0.5823     6.55419162   -14.09750798     8.15201963
q    -0.4226     6.55419162   -12.11925852     3.30898077
q    -0.0251    10.82041217    -9.83128744     6.17423088
q    -0.0006     8.84216271    -9.83128744    11.01726973
q    -0.1003    -2.28797108    -3.27709581    16.74776994
q    -0.8339     0.00000000     0.98912472    13.88251983
q    -0.3281    -4.26622054    -3.27709581    11.90473108
q    -0.3281     4.26622054    -3.27709581    11.90473108
q    -0.1003     2.28797108    -3.27709581    16.74776994
q    -0.1627     0.00000000     5.56506690    13.88251983
q    -0.5681     4.26622054     3.27709581    11.01726973
q    -0.5681    -4.26622054     3.27709581    11.01726973
q    -0.5349     0.00000000     7.54331635     9.03948098
```

```
q    -0.1553    -2.28797108     9.83128744     5.28676952
q    -0.1918     0.00000000    14.09750798     2.42151942
q    -0.2635     0.00000000    12.11925852    -2.42151942
q    -0.4268    -4.26622054     9.83128744     0.44373067
q    -0.4268     4.26622054     9.83128744     0.44373067
q    -0.1553     2.28797108     9.83128744     5.28676952
q    -0.0006    -8.84216271     3.27709581    11.01726973
q    -0.5823    -6.55419162     7.54331635     8.15201963
q    -0.4226    -6.55419162     5.56506690     3.30898077
q    -0.0251   -10.82041217     3.27709581     6.17423088
q    -0.5823     6.55419162     7.54331635     8.15201963
q    -0.4226     6.55419162     5.56506690     3.30898077
q    -0.0251    10.82041217     3.27709581     6.17423088
q    -0.0006     8.84216271     3.27709581    11.01726973
q    -0.1627    -8.84216271    -3.27709581   -11.01726973
q    -0.5681    -6.55419162    -7.54331635    -8.15201963
q    -0.5349   -10.82041217    -3.27709581    -6.17423088
q    -0.8339    -4.26622054    -3.27709581   -11.01726973
q    -0.5681    -6.55419162     0.98912472    -8.15201963
q    -0.3281     0.00000000    -7.54331635    -9.03948098
q    -0.3281     0.00000000     0.98912472    -9.03948098
q    -0.1003     0.00000000    -0.98912472   -13.88251983
q    -0.1003    -0.00000000    -5.56506690   -13.88251983
q    -0.8339     4.26622054    -3.27709581   -11.01726973
q    -0.5681     6.55419162    -7.54331635    -8.15201963
q    -0.5349    10.82041217    -3.27709581    -6.17423088
q    -0.1627     8.84216271    -3.27709581   -11.01726973
q    -0.5681     6.55419162     0.98912472    -8.15201963
q    -0.0251    -6.55419162   -14.09750798    -3.30898077
q    -0.4226    -8.84216271    -9.83128744    -0.44373067
q    -0.0006    -6.55419162   -12.11925852    -8.15201963
q    -0.5823   -10.82041217    -9.83128744    -5.28676952
q    -0.4226    -8.84216271     3.27709581    -0.44373067
q    -0.0251    -6.55419162     7.54331635    -3.30898077
q    -0.0006    -6.55419162     5.56506690    -8.15201963
q    -0.5823   -10.82041217     3.27709581    -5.28676952
q    -0.4268   -13.10838325    -7.54331635     2.42151942
q    -0.2635   -15.39635434    -3.27709581     5.28676952
q    -0.4268   -13.10838325     0.98912472     2.42151942
q    -0.1553   -13.10838325    -0.98912472    -2.42151942
q    -0.1553   -13.10838325    -5.56506690    -2.42151942
q    -0.1918   -17.37460379    -3.27709581     0.44373067
q    -0.0251     6.55419162   -14.09750798    -3.30898077
q    -0.0006     6.55419162   -12.11925852    -8.15201963
q    -0.5823    10.82041217    -9.83128744    -5.28676952
q    -0.4226     8.84216271    -9.83128744    -0.44373067
q    -0.0251     6.55419162     7.54331635    -3.30898077
q    -0.0006     6.55419162     5.56506690    -8.15201963
q    -0.5823    10.82041217     3.27709581    -5.28676952
q    -0.4226     8.84216271     3.27709581    -0.44373067
q    -0.4268    13.10838325    -7.54331635     2.42151942
q    -0.4268    13.10838325     0.98912472     2.42151942
q    -0.1553    13.10838325    -0.98912472    -2.42151942
q    -0.1553    13.10838325    -5.56506690    -2.42151942
q    -0.1918    17.37460379    -3.27709581     0.44373067
q    -0.2635    15.39635434    -3.27709581     5.28676952

# yttrium (NCE)
```

```
basis
Y S
  4.09958000E+00
  3.40192000E+00
  1.29828000E+00
  8.22113000E-01
  3.49905000E-01
Y P
  3.00000000E+00
  1.85000000E+00
  9.17600000E-01
  4.40670000E-01
Y D
  2.35070900E+00
  1.95079200E+00
  6.13000000E-01
end

ecp
Y nelec 39
Y UL
   1    0.582974   -4.001901
Y S
   0    0.231000    6.000000
   1    0.582974    4.001901
Y P
   0    0.141000    5.000000
Y D
   0    3.513290    3.000000
   1    0.419689   -2.765913
   1    0.582974    4.001901
end
```

### B. $YO_8$@CTEP (minimal cluster)

```
# (atomic units)
#     charge         x              y              z

# main cluster

Y     0.0000     0.00000000    -3.27709580     1.43262510
O     0.0000     0.00000000    -7.54331640     2.42151940
O     0.0000    -2.28797110    -3.27709580     5.28676950
O     0.0000     0.00000000     0.98912470     2.42151940
O     0.0000     0.00000000    -0.98912470    -2.42151940
O     0.0000     0.00000000    -5.56506690    -2.42151940
O     0.0000    -4.26622050    -3.27709580     0.44373070
O     0.0000     4.26622050    -3.27709580     0.44373070
O     0.0000     2.28797110    -3.27709580     5.28676950

# nearest cation environment

P     4.0058     0.00000000    -9.83128740     4.29787520
P     3.9036     0.00000000    -3.27709580     7.16312530
P     4.0058     0.00000000     3.27709580     4.29787520
P     3.9036     0.00000000    -3.27709580    -4.29787520
P     4.0058    -6.55419160    -3.27709580    -1.43262510
P     4.0058     6.55419160    -3.27709580    -1.43262510
Y     0.4613     0.00000000    -9.83128740    -1.43262510
Y     0.4613    -6.55419160    -3.27709580     4.29787520
Y     0.4613     0.00000000     3.27709580    -1.43262510
Y     0.4613     6.55419160    -3.27709580     4.29787520

# nearest anion environment

O    -0.2099     0.00000000   -12.11925850     2.42151940
O    -1.6358    -2.28797110    -9.83128740     6.17423090
O    -1.6358     2.28797110    -9.83128740     6.17423090
O    -0.5028     0.00000000    -0.98912470     9.03948100
O    -0.5028     0.00000000    -5.56506690     9.03948100
O    -0.2099     0.00000000     5.56506690     2.42151940
O    -1.6358    -2.28797110     3.27709580     6.17423090
O    -1.6358     2.28797110     3.27709580     6.17423090
O    -0.5028    -2.28797110    -3.27709580    -6.17423090
O    -0.5028     2.28797110    -3.27709580    -6.17423090
O    -1.6358    -6.55419160    -5.56506690    -3.30898080
O    -1.6358    -6.55419160    -0.98912470    -3.30898080
O    -0.2099    -8.84216270    -3.27709580     0.44373070
O    -1.6358     6.55419160    -5.56506690    -3.30898080
O    -1.6358     6.55419160    -0.98912470    -3.30898080
O    -0.2099     8.84216270    -3.27709580     0.44373070

# additional fractional charges

q     0.4077     4.26622050    -9.83128740    -0.44373070
q     0.4077    -4.26622050    -9.83128740    -0.44373070
q     0.4077    -6.55419160    -7.54331640     3.30898080
q     0.4077    -6.55419160     0.98912470     3.30898080
q     0.4077     4.26622050     3.27709580    -0.44373070
q     0.4077    -4.26622050     3.27709580    -0.44373070
q     0.4077     6.55419160    -7.54331640     3.30898080
```

```
q     0.4077     6.55419160     0.98912470     3.30898080


# phosphorus (NCE)
basis
P S
  0.566189
P P
  0.464923
P D
  0.506952
end

ecp
P nelec 15
P UL
   1    6.075091   -6.0293909
P S
   0    0.879676    3.0000000
P P
   0    0.546173    2.0000000
end

# yttrium (NCE)
basis
Y S
  0.349941
Y P
  0.440670
Y D
  0.613096
end

ecp
Y nelec 39
Y UL
   1    0.5829738   -4.0019011
Y S
   0    0.2313380    6.0000000
   1    0.5829738    4.0019011
Y P
   0    0.141219     5.0000000
Y D
   0    3.5130710    3.0000000
   1    0.4196892   -2.7659134
   1    0.5829738    4.0019011
end

# oxygen (NAE)
ecp
O nelec 8
O UL
   2    0.0000001    0.0000000
O S
   0    0.1220650    3.0000000
O P
   0    0.0835810    2.0000000
end
```

### C. $Ce(PO_4)_6$@CTEP (big cluster)

```
# (atomic units)
#     charge         x              y              z

# main cluster

Ce    0.0000     0.00000605    -0.00000014    -0.00000824
P     0.0000    -0.00015385    -6.67199445     2.88327621
P     0.0000    -0.00092546     0.00000835     5.82787606
P     0.0000     0.00036558     6.67200716     2.88324750
P     0.0000    -0.00005847    -0.00004252    -5.81612071
P     0.0000    -6.68698257    -0.00142706    -2.88777872
P     0.0000     6.68715477     0.00145479    -2.88768257
O     0.0000    -0.00047225    -4.39524563     0.98812750
O     0.0000    -2.32960582    -0.00409607     4.01480671
O     0.0000     0.00085538     4.39531453     0.98803290
O     0.0000     0.00525953     2.32753452    -3.99971724
O     0.0000    -0.00540325    -2.32765240    -3.99977067
O     0.0000    -4.41445971    -0.00347964    -0.99306588
O     0.0000     4.41442496     0.00357814    -0.99306751
O     0.0000     2.32791585     0.00411660     4.01500485
O     0.0000     0.00008823    -8.95129308     1.01352263
O     0.0000    -2.28831416    -6.61739460     4.75007405
O     0.0000     2.28841040    -6.61675793     4.74961566
O     0.0000    -0.00340979     2.30041192     7.68165869
O     0.0000     0.00192637    -2.30042477     7.68162245
O     0.0000     0.00017485     8.95134705     1.01354429
O     0.0000    -2.28822991     6.61683971     4.74950956
O     0.0000     2.28848940     6.61726654     4.75013925
O     0.0000    -2.29922288     0.00350239    -7.67125070
O     0.0000     2.29933488    -0.00352760    -7.67104649
O     0.0000    -6.63223681    -2.28927108    -4.75774086
O     0.0000    -6.62978807     2.28790945    -4.75593775
O     0.0000    -8.96995597    -0.00026753    -1.02111963
O     0.0000     6.62992750    -2.28789713    -4.75571681
O     0.0000     6.63244210     2.28929293    -4.75754407
O     0.0000     8.96992235     0.00024785    -1.02080529

# nearest cation environment

Y     2.8313     0.00000605    -6.55419176    -2.86525834
Y     2.8313    -6.55418558    -0.00000014     2.86524186
Y     2.8313     0.00000605     6.55419149    -2.86525834
Y     2.8313     6.55419768    -0.00000014     2.86524186
Y     2.4479     0.00000605   -13.10838339    -0.00000824
Y     2.5682    -6.55418558    -6.55419176     5.73049196
Y     2.6649     0.00000605    -6.55419176     8.59574207
Y     2.5682     6.55419768    -6.55419176     5.73049196
Y     2.5723     0.00000605    -0.00000014    11.46099217
Y     2.6649     0.00000605     6.55419149     8.59574207
Y     2.4479     0.00000605    13.10838312    -0.00000824
Y     2.5682    -6.55418558     6.55419149     5.73049196
Y     2.5682     6.55419768     6.55419149     5.73049196
Y     2.6649    -6.55418558    -0.00000014    -8.59575855
Y     2.5723     0.00000605    -0.00000014   -11.46100865
Y     2.6649     6.55419768    -0.00000014    -8.59575855
Y     2.5682    -6.55418558    -6.55419176    -5.73050845
```

```
Y     2.5682    -6.55418558     6.55419149    -5.73050845
Y     2.4479   -13.10837721    -0.00000014    -0.00000824
Y     2.5682     6.55419768    -6.55419176    -5.73050845
Y     2.5682     6.55419768     6.55419149    -5.73050845
Y     2.4479    13.10838931    -0.00000014    -0.00000824

# additional fractional charges (simulating NAE)

q    -0.8610    -2.28796504    -6.55419176    -6.71940282
q    -0.7580     0.00000605   -10.82041231    -3.85415272
q    -0.6793     4.26622659    -6.55419176    -1.87636397
q    -0.6793    -4.26621449    -6.55419176    -1.87636397
q    -0.8610     2.28797713    -6.55419176    -6.71940282
q    -0.8610    -6.55418558    -2.28797122     6.71938634
q    -0.8610    -6.55418558     2.28797095     6.71938634
q    -0.6793    -6.55418558    -4.26622068     1.87634749
q    -0.7580   -10.82040612    -0.00000014     3.85413624
q    -0.6793    -6.55418558     4.26622041     1.87634749
q    -0.8610    -2.28796504     6.55419149    -6.71940282
q    -0.6793     4.26622659     6.55419149    -1.87636397
q    -0.6793    -4.26621449     6.55419149    -1.87636397
q    -0.8610     2.28797713     6.55419149    -6.71940282
q    -0.7580     0.00000605    10.82041204    -3.85415272
q    -0.8610     6.55419768    -2.28797122     6.71938634
q    -0.8610     6.55419768     2.28797095     6.71938634
q    -0.6793     6.55419768    -4.26622068     1.87634749
q    -0.7580    10.82041822    -0.00000014     3.85413624
q    -0.6793     6.55419768     4.26622041     1.87634749
q    -0.1918     0.00000605   -17.37460394     0.98888614
q    -0.1554    -2.28796504   -13.10838339     3.85413624
q    -0.2635     0.00000605   -15.39635448    -3.85415272
q    -0.4269    -4.26621449   -13.10838339    -0.98890262
q    -0.4269     4.26622659   -13.10838339    -0.98890262
q    -0.1554     2.28797713   -13.10838339     3.85413624
q    -0.5824    -6.55418558   -10.82041231     6.71938634
q    -0.0007    -8.84215667    -6.55419176     9.58463644
q    -0.4226    -6.55418558    -8.84216285     1.87634749
q    -0.0252   -10.82040612    -6.55419176     4.74159759
q    -0.5681    -4.26621449    -6.55419176     9.58463644
q    -0.1627     0.00000605    -8.84216285    12.44988655
q    -0.8340     0.00000605    -4.26622068    12.44988655
q    -0.5349     0.00000605   -10.82041231     7.60684769
q    -0.5681     4.26622659    -6.55419176     9.58463644
q    -0.5824     6.55419768   -10.82041231     6.71938634
q    -0.4226     6.55419768    -8.84216285     1.87634749
q    -0.0252    10.82041822    -6.55419176     4.74159759
q    -0.0007     8.84216876    -6.55419176     9.58463644
q    -0.1004    -2.28796504    -0.00000014    15.31513665
q    -0.8340     0.00000605     4.26622041    12.44988655
q    -0.3282    -4.26621449    -0.00000014    10.47209779
q    -0.3282     4.26622659    -0.00000014    10.47209779
q    -0.1004     2.28797713    -0.00000014    15.31513665
q    -0.1627     0.00000605     8.84216258    12.44988655
q    -0.5681     4.26622659     6.55419149     9.58463644
q    -0.5681    -4.26621449     6.55419149     9.58463644
q    -0.5349     0.00000605    10.82041204     7.60684769
q    -0.1554    -2.28796504    13.10838312     3.85413624
q    -0.1918     0.00000605    17.37460366     0.98888614
```

```
q    -0.2635     0.00000605    15.39635421    -3.85415272
q    -0.4269    -4.26621449    13.10838312    -0.98890262
q    -0.4269     4.26622659    13.10838312    -0.98890262
q    -0.1554     2.28797713    13.10838312     3.85413624
q    -0.0007    -8.84215667     6.55419149     9.58463644
q    -0.5824    -6.55418558    10.82041204     6.71938634
q    -0.4226    -6.55418558     8.84216258     1.87634749
q    -0.0252   -10.82040612     6.55419149     4.74159759
q    -0.5824     6.55419768    10.82041204     6.71938634
q    -0.4226     6.55419768     8.84216258     1.87634749
q    -0.0252    10.82041822     6.55419149     4.74159759
q    -0.0007     8.84216876     6.55419149     9.58463644
q    -0.1627    -8.84215667    -0.00000014   -12.44990303
q    -0.5681    -6.55418558    -4.26622068    -9.58465292
q    -0.5349   -10.82040612    -0.00000014    -7.60686417
q    -0.8340    -4.26621449    -0.00000014   -12.44990303
q    -0.5681    -6.55418558     4.26622041    -9.58465292
q    -0.3282     0.00000605    -4.26622068   -10.47211428
q    -0.3282     0.00000605     4.26622041   -10.47211428
q    -0.1004     0.00000605     2.28797095   -15.31515313
q    -0.1004     0.00000605    -2.28797122   -15.31515313
q    -0.8340     4.26622659    -0.00000014   -12.44990303
q    -0.5681     6.55419768    -4.26622068    -9.58465292
q    -0.5349    10.82041822    -0.00000014    -7.60686417
q    -0.1627     8.84216876    -0.00000014   -12.44990303
q    -0.5681     6.55419768     4.26622041    -9.58465292
q    -0.0252    -6.55418558   -10.82041231    -4.74161407
q    -0.4226    -8.84215667    -6.55419176    -1.87636397
q    -0.0007    -6.55418558    -8.84216285    -9.58465292
q    -0.5824   -10.82040612    -6.55419176    -6.71940282
q    -0.4226    -8.84215667     6.55419149    -1.87636397
q    -0.0252    -6.55418558    10.82041204    -4.74161407
q    -0.0007    -6.55418558     8.84216258    -9.58465292
q    -0.5824   -10.82040612     6.55419149    -6.71940282
q    -0.4269   -13.10837721    -4.26622068     0.98888614
q    -0.2635   -15.39634830    -0.00000014     3.85413624
q    -0.4269   -13.10837721     4.26622041     0.98888614
q    -0.1554   -13.10837721     2.28797095    -3.85415272
q    -0.1554   -13.10837721    -2.28797122    -3.85415272
q    -0.1918   -17.37459775    -0.00000014    -0.98890262
q    -0.0252     6.55419768   -10.82041231    -4.74161407
q    -0.0007     6.55419768    -8.84216285    -9.58465292
q    -0.5824    10.82041822    -6.55419176    -6.71940282
q    -0.4226     8.84216876    -6.55419176    -1.87636397
q    -0.0252     6.55419768    10.82041204    -4.74161407
q    -0.0007     6.55419768     8.84216258    -9.58465292
q    -0.5824    10.82041822     6.55419149    -6.71940282
q    -0.4226     8.84216876     6.55419149    -1.87636397
q    -0.4269    13.10838931    -4.26622068     0.98888614
q    -0.4269    13.10838931     4.26622041     0.98888614
q    -0.1554    13.10838931     2.28797095    -3.85415272
q    -0.1554    13.10838931    -2.28797122    -3.85415272
q    -0.1918    17.37460985    -0.00000014    -0.98890262
q    -0.2635    15.39636039    -0.00000014     3.85413624

(see the Y(PO4)6@CTEP big cluster for CTPPs and basis sets on pseudoatoms)
```

### D. $CeO_8$@CTEP (minimal cluster)

```
# (atomic units)
#     charge         x              y              z

# main cluster

Ce    0.0000     0.00038238    -0.00111199    -2.91078546
O     0.0000     0.00039012    -4.40836268    -1.92935293
O     0.0000    -2.32258349    -0.00123598     1.09609842
O     0.0000     0.00039162     4.40606607    -1.92937165
O     0.0000     0.00039252     2.32171200    -6.91771962
O     0.0000     0.00038548    -2.32422336    -6.91773833
O     0.0000    -4.40666672    -0.00113295    -3.89259004
O     0.0000     4.40740836    -0.00113992    -3.89262244
O     0.0000     2.32334459    -0.00123547     1.09610223

# nearest cation environment

P     3.7544     0.00038479    -6.67800963    -0.02801295
P     4.7118     0.00038863    -0.00116829     2.91610282
P     3.6514     0.00038489     6.67572789    -0.02804467
P     4.5829     0.00038554    -0.00124298    -8.73769523
P     3.8647    -6.67653241    -0.00110958    -5.79364687
P     3.8582     6.67727989    -0.00111186    -5.79364045
Y     0.7204     0.00038238    -6.55530362    -5.77603557
Y     0.7204    -6.55380925    -0.00111199    -0.04553536
Y     0.7204     0.00038238     6.55307964    -5.77603557
Y     0.7204     6.55457401    -0.00111199    -0.04553536

# nearest anion environment

O     0.0514     0.00038434    -8.96361317    -1.89048464
O    -1.1462    -2.28770558    -6.61861235     1.84075884
O    -1.1611     2.28847222    -6.61860836     1.84075702
O    -1.5362     0.00038425     2.29776690     4.77115746
O    -1.4189     0.00038483    -2.30000122     4.77128258
O     0.1160     0.00038171     8.96132994    -1.89052244
O    -1.0383    -2.28771009     6.61632275     1.84071168
O    -0.9682     2.28847741     6.61632269     1.84070899
O    -1.3202    -2.29850805    -0.00120846   -10.59282281
O    -1.3178     2.29927275    -0.00121305   -10.59282282
O    -1.2279    -6.61741558    -2.28918661    -7.66243237
O    -1.2872    -6.61731829     2.28698578    -7.66241158
O    -0.0143    -8.96192624    -0.00108090    -3.93089450
O    -1.2379     6.61818683    -2.28918647    -7.66243508
O    -1.2411     6.61808827     2.28698501    -7.66240595
O     0.0053     8.96267486    -0.00108463    -3.93087015

# additional fractional charges

q     0.0613     0.00038238   -13.10949525    -2.91078546
q     0.0613    -6.55380925    -6.55530362     2.81971474
q     0.0613     0.00038238    -6.55530362     5.68496485
q     0.0613     6.55457401    -6.55530362     2.81971474
q     0.0613     0.00038238    -0.00111199     8.55021495
q     0.0613     0.00038238     6.55307964     5.68496485
q     0.0613     0.00038238    13.10727127    -2.91078546
```

```
q     0.0613    -6.55380925     6.55307964     2.81971474
q    -0.0527     6.55457401     6.55307964     2.81971474
```

(see the YO8@CTEP minimal cluster for CTPPs and basis sets on pseudoatoms)

### E. Th$(PO_4)_6$@CTEP (big cluster)

```
# (atomic units)
#     charge        x              y              z

# main cluster

Th    0.0000    -0.00000000    -0.00000003    -0.00000000
P     0.0000    -0.00002184    -6.73288595     2.91318464
P     0.0000    -0.00000772     0.00000383     5.87302196
P     0.0000     0.00002299     6.73286636     2.91317386
P     0.0000     0.00000118     0.00004404    -5.87296736
P     0.0000    -6.73299404    -0.00002988    -2.91340574
P     0.0000     6.73299470     0.00001403    -2.91340419
O     0.0000    -0.00004475    -4.45231886     1.02301869
O     0.0000    -2.33143197     0.00003995     4.05705121
O     0.0000     0.00004554     4.45230382     1.02300087
O     0.0000    -0.00001768     2.33142334    -4.05693392
O     0.0000     0.00001775    -2.33135607    -4.05696757
O     0.0000    -4.45228941    -0.00005845    -1.02347899
O     0.0000     4.45229101     0.00003061    -1.02347561
O     0.0000     2.33141862     0.00000481     4.05705533
O     0.0000    -0.00000482    -9.00136623     1.03626307
O     0.0000    -2.28999109    -6.66779961     4.77821107
O     0.0000     2.28996189    -6.66775983     4.77819251
O     0.0000     0.00000479     2.30644725     7.71622473
O     0.0000    -0.00001899    -2.30646516     7.71618761
O     0.0000     0.00000447     9.00135043     1.03625939
O     0.0000    -2.28995951     6.66773164     4.77818068
O     0.0000     2.28999381     6.66777241     4.77819493
O     0.0000    -2.30642981     0.00004151    -7.71609026
O     0.0000     2.30643401     0.00006589    -7.71608736
O     0.0000    -6.66802196    -2.29000454    -4.77847444
O     0.0000    -6.66798215     2.28996538    -4.77844628
O     0.0000    -9.00140526    -0.00001332    -1.03639821
O     0.0000     6.66798253    -2.28997421    -4.77845581
O     0.0000     6.66802256     2.28999614    -4.77846118
O     0.0000     9.00140601    -0.00000399    -1.03639668

# nearest cation environment

Y     2.8312    -0.00000000    -6.55419165    -2.86525010
Y     2.8312    -6.55419163    -0.00000003     2.86525010
Y     2.8312    -0.00000000     6.55419160    -2.86525010
Y     2.8312     6.55419163    -0.00000003     2.86525010
Y     2.4478    -0.00000000   -13.10838328    -0.00000000
Y     2.5681    -6.55419163    -6.55419165     5.73050020
Y     2.6649    -0.00000000    -6.55419165     8.59575031
Y     2.5681     6.55419163    -6.55419165     5.73050020
Y     2.5722    -0.00000000    -0.00000003    11.46100041
Y     2.6649    -0.00000000     6.55419160     8.59575031
Y     2.4478    -0.00000000    13.10838323    -0.00000000
Y     2.5681    -6.55419163     6.55419160     5.73050020
Y     2.5681     6.55419163     6.55419160     5.73050020
Y     2.6649    -6.55419163    -0.00000003    -8.59575031
Y     2.5722    -0.00000000    -0.00000003   -11.46100041
Y     2.6649     6.55419163    -0.00000003    -8.59575031
Y     2.5681    -6.55419163    -6.55419165    -5.73050021
```

```
Y     2.5681    -6.55419163     6.55419160    -5.73050021
Y     2.4478   -13.10838326    -0.00000003    -0.00000000
Y     2.5681     6.55419163    -6.55419165    -5.73050021
Y     2.5681     6.55419163     6.55419160    -5.73050021
Y     2.4478    13.10838326    -0.00000003    -0.00000000

# additional fractional charges (simulating NAE)

q    -0.8610    -2.28797109    -6.55419165    -6.71939458
q    -0.7580    -0.00000000   -10.82041220    -3.85414448
q    -0.6793     4.26622054    -6.55419165    -1.87635573
q    -0.6793    -4.26622054    -6.55419165    -1.87635573
q    -0.8610     2.28797108    -6.55419165    -6.71939458
q    -0.8610    -6.55419163    -2.28797111     6.71939458
q    -0.8610    -6.55419163     2.28797106     6.71939458
q    -0.6793    -6.55419163    -4.26622057     1.87635573
q    -0.7580   -10.82041217    -0.00000003     3.85414448
q    -0.6793    -6.55419163     4.26622052     1.87635573
q    -0.8610    -2.28797109     6.55419160    -6.71939458
q    -0.6793     4.26622054     6.55419160    -1.87635573
q    -0.6793    -4.26622054     6.55419160    -1.87635573
q    -0.8610     2.28797108     6.55419160    -6.71939458
q    -0.7580    -0.00000000    10.82041215    -3.85414448
q    -0.8610     6.55419163    -2.28797111     6.71939458
q    -0.8610     6.55419163     2.28797106     6.71939458
q    -0.6793     6.55419163    -4.26622057     1.87635573
q    -0.7580    10.82041217    -0.00000003     3.85414448
q    -0.6793     6.55419163     4.26622052     1.87635573
q    -0.1918    -0.00000000   -17.37460383     0.98889438
q    -0.1554    -2.28797109   -13.10838328     3.85414448
q    -0.2635    -0.00000000   -15.39635437    -3.85414448
q    -0.4269    -4.26622054   -13.10838328    -0.98889438
q    -0.4269     4.26622054   -13.10838328    -0.98889438
q    -0.1554     2.28797108   -13.10838328     3.85414448
q    -0.5824    -6.55419163   -10.82041220     6.71939458
q    -0.0007    -8.84216272    -6.55419165     9.58464468
q    -0.4226    -6.55419163    -8.84216274     1.87635573
q    -0.0252   -10.82041217    -6.55419165     4.74160583
q    -0.5681    -4.26622054    -6.55419165     9.58464468
q    -0.1627    -0.00000000    -8.84216274    12.44989479
q    -0.8340    -0.00000000    -4.26622057    12.44989479
q    -0.5349    -0.00000000   -10.82041220     7.60685593
q    -0.5681     4.26622054    -6.55419165     9.58464468
q    -0.5824     6.55419163   -10.82041220     6.71939458
q    -0.4226     6.55419163    -8.84216274     1.87635573
q    -0.0252    10.82041217    -6.55419165     4.74160583
q    -0.0007     8.84216271    -6.55419165     9.58464468
q    -0.1004    -2.28797109    -0.00000003    15.31514489
q    -0.8340    -0.00000000     4.26622052    12.44989479
q    -0.3282    -4.26622054    -0.00000003    10.47210603
q    -0.3282     4.26622054    -0.00000003    10.47210603
q    -0.1004     2.28797108    -0.00000003    15.31514489
q    -0.1627    -0.00000000     8.84216269    12.44989479
q    -0.5681     4.26622054     6.55419160     9.58464468
q    -0.5681    -4.26622054     6.55419160     9.58464468
q    -0.5349    -0.00000000    10.82041215     7.60685593
q    -0.1554    -2.28797109    13.10838323     3.85414448
q    -0.1918    -0.00000000    17.37460377     0.98889438
```

```
q    -0.2635    -0.00000000    15.39635432    -3.85414448
q    -0.4269    -4.26622054    13.10838323    -0.98889438
q    -0.4269     4.26622054    13.10838323    -0.98889438
q    -0.1554     2.28797108    13.10838323     3.85414448
q    -0.0007    -8.84216272     6.55419160     9.58464468
q    -0.5824    -6.55419163    10.82041215     6.71939458
q    -0.4226    -6.55419163     8.84216269     1.87635573
q    -0.0252   -10.82041217     6.55419160     4.74160583
q    -0.5824     6.55419163    10.82041215     6.71939458
q    -0.4226     6.55419163     8.84216269     1.87635573
q    -0.0252    10.82041217     6.55419160     4.74160583
q    -0.0007     8.84216271     6.55419160     9.58464468
q    -0.1627    -8.84216272    -0.00000003   -12.44989479
q    -0.5681    -6.55419163    -4.26622057    -9.58464468
q    -0.5349   -10.82041217    -0.00000003    -7.60685593
q    -0.8340    -4.26622054    -0.00000003   -12.44989479
q    -0.5681    -6.55419163     4.26622052    -9.58464468
q    -0.3282    -0.00000000    -4.26622057   -10.47210604
q    -0.3282    -0.00000000     4.26622052   -10.47210604
q    -0.1004    -0.00000000     2.28797106   -15.31514489
q    -0.1004    -0.00000000    -2.28797111   -15.31514489
q    -0.8340     4.26622054    -0.00000003   -12.44989479
q    -0.5681     6.55419163    -4.26622057    -9.58464468
q    -0.5349    10.82041217    -0.00000003    -7.60685593
q    -0.1627     8.84216271    -0.00000003   -12.44989479
q    -0.5681     6.55419163     4.26622052    -9.58464468
q    -0.0252    -6.55419163   -10.82041220    -4.74160583
q    -0.4226    -8.84216272    -6.55419165    -1.87635573
q    -0.0007    -6.55419163    -8.84216274    -9.58464468
q    -0.5824   -10.82041217    -6.55419165    -6.71939458
q    -0.4226    -8.84216272     6.55419160    -1.87635573
q    -0.0252    -6.55419163    10.82041215    -4.74160583
q    -0.0007    -6.55419163     8.84216269    -9.58464468
q    -0.5824   -10.82041217     6.55419160    -6.71939458
q    -0.4269   -13.10838326    -4.26622057     0.98889438
q    -0.2635   -15.39635435    -0.00000003     3.85414448
q    -0.4269   -13.10838326     4.26622052     0.98889438
q    -0.1554   -13.10838326     2.28797106    -3.85414448
q    -0.1554   -13.10838326    -2.28797111    -3.85414448
q    -0.1918   -17.37460380    -0.00000003    -0.98889438
q    -0.0252     6.55419163   -10.82041220    -4.74160583
q    -0.0007     6.55419163    -8.84216274    -9.58464468
q    -0.5824    10.82041217    -6.55419165    -6.71939458
q    -0.4226     8.84216271    -6.55419165    -1.87635573
q    -0.0252     6.55419163    10.82041215    -4.74160583
q    -0.0007     6.55419163     8.84216269    -9.58464468
q    -0.5824    10.82041217     6.55419160    -6.71939458
q    -0.4226     8.84216271     6.55419160    -1.87635573
q    -0.4269    13.10838326    -4.26622057     0.98889438
q    -0.4269    13.10838326     4.26622052     0.98889438
q    -0.1554    13.10838326     2.28797106    -3.85414448
q    -0.1554    13.10838326    -2.28797111    -3.85414448
q    -0.1918    17.37460380    -0.00000003    -0.98889438
q    -0.2635    15.39635434    -0.00000003     3.85414448
```

(see the Y(PO4)6@CTEP big cluster for CTPPs and basis sets on pseudoatoms)

### F. $ThO_8$@CTEP (minimal cluster)

```
# (atomic units)
#     charge         x              y              z

# main cluster

Th    0.0000    -0.00000000    -0.00000003    -0.00000000
O     0.0000    -0.00004475    -4.45231886     1.02301869
O     0.0000    -2.33143197     0.00003995     4.05705121
O     0.0000     0.00004554     4.45230382     1.02300087
O     0.0000    -0.00001768     2.33142334    -4.05693392
O     0.0000     0.00001775    -2.33135607    -4.05696757
O     0.0000    -4.45228941    -0.00005845    -1.02347899
O     0.0000     4.45229101     0.00003061    -1.02347561
O     0.0000     2.33141862     0.00000481     4.05705533

# nearest cation environment

P     4.0932    -0.00002184    -6.73288595     2.91318464
P     4.4046    -0.00000772     0.00000383     5.87302196
P     4.0303     0.00002299     6.73286636     2.91317386
P     4.3571     0.00000118     0.00004404    -5.87296736
P     4.0553    -6.73299404    -0.00002988    -2.91340574
P     4.0365     6.73299470     0.00001403    -2.91340419
Y     1.2246    -0.00000000    -6.55419165    -2.86525010
Y     1.2246    -6.55419163    -0.00000003     2.86525010
Y     1.2246    -0.00000000     6.55419160    -2.86525010
Y     1.2246     6.55419163    -0.00000003     2.86525010

# nearest anion environment

O    -0.3188    -0.00000482    -9.00136623     1.03626307
O    -1.3514    -2.28999109    -6.66779961     4.77821107
O    -1.3433     2.28996189    -6.66775983     4.77819251
O    -0.9890     0.00000479     2.30644725     7.71622473
O    -0.9860    -0.00001899    -2.30646516     7.71618761
O    -0.2507     0.00000447     9.00135043     1.03625939
O    -1.3372    -2.28995951     6.66773164     4.77818068
O    -1.3278     2.28999381     6.66777241     4.77819493
O    -0.9615    -2.30642981     0.00004151    -7.71609026
O    -0.9423     2.30643401     0.00006589    -7.71608736
O    -1.3406    -6.66802196    -2.29000454    -4.77847444
O    -1.2913    -6.66798215     2.28996538    -4.77844628
O    -0.3098    -9.00140526    -0.00001332    -1.03639821
O    -1.3420     6.66798253    -2.28997421    -4.77845581
O    -1.2670     6.66802256     2.28999614    -4.77846118
O    -0.3099     9.00140601    -0.00000399    -1.03639668

# additional fractional charges

q    -0.1561    -4.26622054     6.55419160    -1.87635573
q    -0.1561     4.26622054     6.55419160    -1.87635573
q    -0.1561     6.55419163     4.26622052     1.87635573
q    -0.1561    -6.55419163     4.26622052     1.87635573
q    -0.1561    -6.55419163    -4.26622057     1.87635573
q    -0.1561     6.55419163    -4.26622057     1.87635573
q    -0.1561     4.26622054    -6.55419165    -1.87635573
```

```
q    -0.1561    -4.26622054    -6.55419165    -1.87635573
q     0.0424     2.28797108     6.55419160    -6.71939458
```

(see the YO8@CTEP minimal cluster for CTPPs and basis sets on pseudoatoms)

## III. PSEUDOPOTENTIALS AND BASIS SETS THE FOR MAIN CLUSTER

### A. RPP and basis sets for DFT calculations

```
# yttrium (main cluster)
Y S
  4.0995800000
  3.4019200000
  1.2982800000
  0.8221130000
  0.3499050000
Y P
  3.0000000000
  1.8500000000
  0.9176000000
  0.4406700000
Y D
  2.3507090000
  1.9507920000
  0.6130000000
end

ecp
Y nelec 28
Y UL
   1   11.81593920  -12.91092320
   2    5.59889380  -11.18022840
   2    2.06957630   -0.85744630
   2    1.43175820    0.14792800
   2    0.97068170   -0.02292530
Y S
   0   20.03228840    6.00000000
   1    6.42648610  194.36171420
   1    4.68991600 -350.17035040
   1    3.37947590  330.47086400
   1    1.17384470 -159.06590280
   2    1.39456800  163.34692920
   2    0.66958510    2.22322580
   2    0.44326850   -0.34080310
   2    0.27350830    0.01667880
Y P
   0    6.35135940    5.00000000
   1    9.25965370   16.35956370
   2    2.40646250   87.70585300
   2    1.74971080  -93.62824730
   2    1.26879800   54.35195790
   2    0.91212170  -20.44031200
   2    0.64863110    5.08534270
   2    0.45450400   -0.77712730
   2    0.31151540    0.05389480
Y D
   0    0.58493070    3.00000000
   1   10.59573490    9.82547590
   1    4.44225910    4.52886520
   1    1.44402090    1.46088210
   2    0.85506720   -2.36136650
end
```

```
# cerium (main cluster)
basis
Ce  S
  38.132735834       1.0000000000
  32.845141012      -1.0934516135
  22.992538344      -4.0320861015
  17.097574146       15.048267619
  12.147307085      -17.565404206
  3.0368466172       9.8719630535
Ce  S
  1.5641239751
 0.61546672586
 0.28394827461
 0.20394308153
Ce  P
  9.6063846059      1.00000000000      1.0000000000
  8.6349737937     -0.64518392813     -0.0073015658
  4.1785893262     -1.00312823380     -2.2124709894
  1.8790757759     -0.74487188536     -1.8186319244
Ce  P
 0.70678680542
 0.27927026535
Ce  D
  23.336013720
  5.5814615442
  2.6541395941
  1.1106024799
 0.29834105859
 0.05534499287
Ce  F
  146.13971234
  108.52865126
  27.595534817
  9.4317556135
  3.4221355199
  1.1490074773
  0.3378567167
end

ecp
Ce nelec 28
Ce UL
   1        148.2339873          8.5858608
   1        110.6492831        -14.6515890
   1         27.8114419         -9.6584770
   1          9.7218360         -1.5578802
   1          1.0850681          0.0231752
   2          0.9230271          0.0041175
Ce S
   0        222.2708777          6.0000000
   1         96.8679966         53.1181626
   2        126.0026363        613.7607828
   2         30.0218033       1560.5447343
   2         22.1519973      -2239.7523511
   2         16.4819907       1539.3581624
   2         12.0734762       -209.8427650
   2          1.5286717         -0.0550817
   2          0.5831509         -0.0051044
```

```
Ce P
   0          0.2545400         5.0000000
   1         37.2881309       -12.3475943
   1         24.0922652       110.9509765
   1         15.8161826      -248.3838941
   1         10.8545877       187.7543345
   2          5.8452265      -155.7971505
   2          4.1222970        92.9770501
   2          2.8752808       -40.6660833
   2          0.8247982        -4.1549047
   2          0.3457197        -1.1814669
   2          0.1356527        -0.0051954
Ce D
   0         26.0321704         3.0000000
   1          5.1583391        23.0044121
   1          2.6115110         9.5369149
   2          4.5134309       -49.7002470
   2          1.7821766        -2.2392985
   2          1.2464941         0.3054215
end

# thorium (main cluster)
basis
Th  S
  9.9454800000      -1.5692679640
  7.3670200000       4.1978018020
  5.6247000000      -2.2362318800
Th  S
  2.1776480000
  1.5434900000
 0.68138000000
 0.26921000000
Th  P
  12.148523596     -0.08742472500
  8.0990157307      0.44806707400
  5.3993438205     -0.32054202600
Th  P
  12.148523596     -0.07611783800
  8.0990157307      0.26583164500
  5.3993438205      0.00688897400
Th  P
  2.5538500000
  1.1935000000
 0.48203000000
 0.19281000000
Th  D
  9.1698776226      0.04492841908
  3.8464227235      0.15024177255
  1.5399500000     -0.31869000000
Th  D
  3.3762700000
 0.68138000000
 0.26922000000
Th  F
  3.5253810000      0.12955054200
  1.3309050000      0.27512146700
Th  F
 0.48203490000
```

```
 0.19281396000
end

ecp
Th nelec 60
Th ul
   1         369.8978299          40.1688625
   1         247.7655967         -75.8400918
   2         201.1047072        1119.1256179
   2         149.6430016        -939.0212475
   2          46.4082035        -158.9114783
   2          33.2131211          54.3490910
   2          23.2792483        -103.6155449
   2          12.0974369         -21.4878949
   2           6.7154251          -4.6231764
   2           3.7306700          -0.4213014
Th S
   0         185.6149913          10.0000000
   1          72.6961055        1665.6899240
   1          50.6204540       -3162.4093964
   1          24.4565158        1544.8455643
   2          45.0670100       16686.0356712
   2          32.3639658      -22838.9890953
   2          23.4734928       17122.9705699
   2          17.0092082      -16493.0116439
   2          12.2600499       11122.5206143
   2           8.8074716       -5533.3540253
   2           6.3034875        2410.7028178
   2           4.4810123        -951.2552943
   2           3.1537158         342.8842982
   2           2.1927606        -112.5329044
   2           1.5033497          32.7476657
   2           1.0158387          -8.1584578
   2           0.6773387           1.6382610
   2           0.4466685          -0.2396255
   2           0.2906293           0.0179686
Th P
   0          33.6223842           9.0000000
   1         108.6498486         -10.4601943
   1          63.4425062          32.0830066
   1          37.5250819          50.9637244
   1          23.8235078        -145.7224291
   1          14.2239613         119.5147818
   2          17.2497787        1296.8254441
   2          12.1926689       -2669.8125901
   2           8.7994523        2764.0417149
   2           6.4045302       -1592.8038416
   2           4.5979338         655.5382879
   2           3.2347665        -209.3159925
   2           2.2306039          52.2880878
   2           1.4870307          -8.9660732
   2           0.7071097           0.8286893
   2           0.3868824          -0.2886767
   2           0.2269165           0.1169487
   2           0.1375627          -0.0393963
Th D
   0          47.0650006           7.0000000
   1          44.6652085          44.8594927
```

```
   2          21.4155025         283.8219406
   2           5.6703091         180.1522228
   2           4.0517413        -103.0854171
   2           2.6438191          31.9011410
   2           1.6754047          -9.7884334
   2           1.1196517           3.0761092
   2           0.7541756          -0.6618045
   2           0.5018691           0.0727947
Th F
   0          43.5950107           4.0000000
   1          27.4891244          48.5573039
   2          10.7795340         142.2668629
   2           2.0985194          17.9345386
   2           1.4899767         -15.5961935
   2           1.0503853           6.0455554
   2           0.7271426          -1.1084923
   2           0.4904562           0.0730222
end

# oxygen (main cluster)
basis
O S
  27032.382631     0.21726302465E-03
  4052.3871392     0.16838662199E-02
  922.32722710     0.87395616265E-02
  261.24070989     0.35239968808E-01
  85.354641351     0.11153519115
  31.035035245     0.25588953961
O S
  12.260860728     0.39768730901
   4.998707601     0.24627849430
O S
   1.098713600
   0.356587010
O P
  63.274954801     0.60685103418E-02
  14.627049379     0.41912575824E-01
  4.4501223456     0.16153841088
  1.5275799647     0.35706951311
O P
  0.5489735000
  0.1858671100
O D
  0.2534621300
end

# phosphorus (main cluster)
basis
P S
  5.24269992E+04  0.000535
  7.86326606E+03  0.004137
  1.78952273E+03  0.021257
  5.06273002E+02  0.083030
  1.64606985E+02  0.240761
  5.83919187E+01  0.449106
  2.16436632E+01  0.342625
P S
  9.90138376E+01  0.088204
```

```
  3.05504398E+01  0.385317
  5.45370877E+00 -1.186532
P S
  2.65033626E+00  0.682258
  1.27266889E+00  0.339268
P S
  3.07240970E-01
  1.10270830E-01
P P
  4.72272192E+02  0.003644
  1.11588828E+02  0.028701
  3.54459364E+01  0.129799
  1.29907769E+01  0.364950
  5.04862217E+00  0.607502
P P
  1.88897552E+00
  4.42406420E-01
  1.57322530E-01
P D
  5.06129500E-01
end
```

### B. RPP and basis set for cerium (FS-RCC calculations)

```
basis
Ce S
        54.39885600   -0.02521881    0.01548137    0.01678920
        33.01586900    0.13580583   -0.08533010   -0.08147980
        20.34342600   -0.44759878    0.31914646    0.37029245
        12.90826400    0.40723739   -0.41329217   -0.46630731
         7.98930370    0.83594647   -0.38759894   -1.26212362
         4.60449000   -0.64725056    0.35120848    2.12959809
         2.79405100   -0.42970833    0.59872206    0.59748125
         1.66457470   -0.56643592    0.67314587    0.49552501
         0.96559745    0.06807410   -0.25601840   -3.02390818
         0.54472461   -0.15583120   -0.69980135    0.07123842
         0.30843128    0.02327782   -0.51965302    1.25659880
         0.17091904   -0.04038428   -0.03703799    0.30871151
         0.09595563    0.01791068   -0.01200308   -0.01775593
         0.05034068   -0.00647612    0.00455803    0.00650131
         0.02687818    0.00147866   -0.00108641   -0.00133032
Ce P
        53.76593900    0.00173934   -0.00195223    0.01089766   -0.02198755
        30.00471500    0.00566716    0.00238599   -0.04636265    0.10678718
        17.09649800   -0.03876557   -0.00084199    0.17414300   -0.41792705
         9.88498630    0.39157690   -0.20856136    0.26101337   -0.23216015
         5.73120520   -0.37499072    0.25270339   -1.03898223    2.43778153
         3.25595870   -0.43628385    0.33718223   -0.28530536   -1.11384659
         1.85207290   -0.38864129    0.31130730    0.22916463   -1.78277377
         1.03078900   -0.05291303   -0.22902229    1.15414370    0.77449334
         0.56080336   -0.07905623   -0.51807667    0.06447889    1.63366853
         0.30599502   -0.01597604   -0.41805553   -0.68524460   -0.92411348
         0.16623214   -0.01669819   -0.06869580   -0.32420761   -0.42367009
         0.08302680    0.00492144   -0.00645790    0.00329111   -0.05476563
         0.04253647   -0.00227937    0.00259499   -0.00509085    0.01818866
         0.02187241    0.00061893   -0.00073463    0.00137576   -0.00494447
Ce D
        33.95121700    0.00790301   -0.00366881   -0.01595412    0.02979929
        19.07349500    0.00137710   -0.00004921    0.03592263   -0.07246385
        10.81853100    0.01718145   -0.00775534   -0.13115437    0.21776061
         6.10664820   -0.26552094    0.13733545    0.61794157   -1.30696810
         3.38363550   -0.41106391    0.17892599    0.27116997    0.38353168
         1.84969960   -0.33050477    0.12371488   -0.25407288    1.38514136
         0.97563290   -0.11707543   -0.20764636   -0.84401518   -0.68115581
         0.47143369   -0.01417732   -0.48402501    0.03082864   -0.92509966
         0.21920994    0.00082755   -0.41121426    0.60853344    0.76550605
         0.09783436   -0.00044646   -0.08410660    0.13574544    0.18464540
         0.04118330    0.00012374    0.00254849   -0.00302513   -0.00027441
Ce F
       443.94603000   -0.00013708   -0.00005312    0.00011935
       153.68283000   -0.00181082   -0.00169696   -0.00388219
        65.78857500   -0.00932696   -0.00515728   -0.00112876
        31.40169000   -0.03315030   -0.03079258   -0.06996321
        15.70903700   -0.08303991   -0.03269181    0.03726415
         8.17887530   -0.18069547   -0.25080921   -0.65912121
         4.31368970   -0.27792691   -0.42970271   -0.17182205
         2.26695420   -0.28946126   -0.11842287    0.87028667
         1.17381240   -0.26012063    0.40438379    0.30296557
         0.58896033   -0.18638613    0.45485914   -0.59105820
         0.28109557   -0.07618368    0.11990144   -0.22866659
```

```
          0.12108258   -0.00795985    0.01201019   -0.01782442
          0.05215661    0.00034491   -0.00128137    0.00110360
Ce G
         24.00000000    0.02519062   -0.03351364
         12.00000000    0.03111841   -0.04268626
          6.00000000    0.39144383   -0.51814627
          3.00000000    0.30570379   -0.25997620
          1.50000000    0.29860507    0.33102324
          0.75000000    0.24534762    0.54268882
          0.37500000    0.04782811    0.10240751
Ce H
         14.80000000   -0.00542043
          7.40000000    0.41309467
          3.70000000    0.38579042
          1.85000000    0.27462181
          0.92500000    0.21752991
          0.46250000    0.03429413
end

ecp
Ce nelec 28
Ce UL
   1      1.482339873341e+02      8.585860822513e+00
   1      1.106492831019e+02     -1.465158903629e+01
   1      2.781144191195e+01     -9.658477034314e+00
   1      9.721836011083e+00     -1.557880182653e+00
   1      1.085068094798e+00      2.317518572450e-02
   2      9.230270964281e-01      4.117510812879e-03
Ce S
   0      2.222708777449e+02      6.000000000000e+00
   1      9.686799659022e+01      5.311816255338e+01
   2      1.260026363341e+02      6.137607828354e+02
   2      3.002180332591e+01      1.560544734253e+03
   2      2.215199731549e+01     -2.239752351094e+03
   2      1.648199066263e+01      1.539358162445e+03
   2      1.207347616043e+01     -2.098427649533e+02
   2      1.528671720974e+00     -5.508170789995e-02
   2      5.831508966501e-01     -5.104383160047e-03
Ce P
   0      2.545400050672e-01      5.000000000000e+00
   1      3.728813090161e+01     -1.234759430746e+01
   1      2.409226522067e+01      1.109509764977e+02
   1      1.581618258941e+01     -2.483838941131e+02
   1      1.085458766493e+01      1.877543344522e+02
   2      5.845226534485e+00     -1.557971504727e+02
   2      4.122296990636e+00      9.297705014556e+01
   2      2.875280795544e+00     -4.066608334266e+01
   2      8.247981837772e-01     -4.154904684264e+00
   2      3.457196703582e-01     -1.181466870868e+00
   2      1.356526512904e-01     -5.195364393874e-03
   2      5.724205934841e-02      1.308651620526e-04
Ce D
   0      2.603217037510e+01      3.000000000000e+00
   1      5.158339108309e+00      2.300441214388e+01
   1      2.611511037675e+00      9.536914946237e+00
   2      4.513430912971e+00     -4.970024701338e+01
   2      1.782176553898e+00     -2.239298546264e+00
   2      1.246494109966e+00      3.054214914790e-01
```

```
   2      4.542278372778e-03      3.649564744413e-06
end

so
Ce P
   1      3.728813090161e+01     -7.639495534208e+00
   1      2.409226522067e+01      2.652678550000e+01
   1      1.581618258941e+01     -3.379061471970e+01
   1      1.085458766493e+01      1.531244470684e+01
   2      5.845226534485e+00      5.243275098674e+00
   2      4.122296990636e+00     -4.244396071515e+00
   2      2.875280795544e+00      1.006814164840e+00
   2      8.247981837772e-01     -1.073961517519e-02
   2      3.457196703582e-01     -1.168237464337e-04
   2      1.356526512904e-01      2.752200922718e-06
   2      5.724205934841e-02      1.969481865094e-06
Ce D
   1      5.158339108309e+00      2.415081237487e-01
   1      2.611511037675e+00     -2.189988145563e-01
   2      4.513430912971e+00      5.095607797611e-01
   2      1.782176553898e+00      8.117431444005e-02
   2      1.246494109966e+00     -1.941747476972e-02
   2      4.542278372778e-03      5.760701418937e-07
Ce F
   1      1.482339873341e+02     -6.917575818079e-01
   1      1.106492831019e+02      1.423511529183e+00
   1      2.781144191195e+01      4.142392620582e-03
   1      9.721836011083e+00      1.062759933185e-02
   1      1.085068094798e+00     -3.396992231006e-04
   2      9.230270964281e-01      1.049033295916e-03
end
```

### C. RPP and basis set for thorium (FS-RCC calculations)

```
basis
Th S
          9.94548000    1.58334466    1.23107610    0.42185745   -1.01542176
          7.36702000   -4.09864134   -3.52731002   -1.23993211    3.06257426
          5.62470000    2.06605424    2.11914883    0.77230956   -1.97362892
          2.17765000    0.75727333    0.48125809    0.16896935   -1.00498648
          1.54349000    0.32293945    0.90509192    0.39427397    0.01298937
          0.68138000    0.12288675   -0.95950300   -0.55301063    1.73766617
          0.26921000    0.04551568   -0.71572307   -0.68141935   -0.19919127
          0.10769000   -0.00103455    0.04669139    0.54158842   -1.87748653
          0.04308000    0.00117865   -0.03651208    0.79074742    0.87991479
          0.01723000   -0.00064083    0.01627762    0.07723938    0.62601911
          0.00689200    0.00018327   -0.00470805    0.00072105   -0.05459072
Th P
         12.14852000    0.13547132   -0.06802470   -0.06085799    0.21807023
          8.09902000   -0.55349438    0.32650584    0.30413281   -1.08027083
          5.39934000    0.18129869   -0.14699461   -0.17054514    0.93376420
          2.55385000    0.79672970   -0.59835726   -0.60005825    1.33310215
          1.19350000    0.32367288   -0.09736500    0.28270715   -1.91188311
          0.48203000    0.03757171    0.78889994    0.76920412    0.15126083
          0.19281000    0.01555003    0.38787720   -0.32838428    1.34646751
          0.07712600   -0.00088360    0.00004548   -0.74699625   -0.98448647
          0.03085000    0.00073938    0.00870053   -0.12922178   -0.11804204
          0.01234000   -0.00023402   -0.00271516    0.00379658   -0.01796934
Th D
         19.37309000    0.00691280    0.00324599   -0.00905872    0.02011389
          7.49914000    0.10066612    0.03248481   -0.11161890    0.14918526
          3.30747000   -0.45425449   -0.17952011    0.70501699   -1.28441508
          1.56760000   -0.54532188   -0.20026190    0.06899259    1.16807190
          0.68138000   -0.16103427    0.16721054   -0.91526457    0.23035537
          0.26922000   -0.00067816    0.53358715   -0.07413489   -1.01465265
          0.10769000   -0.00247220    0.41709042    0.54272016    0.37344344
          0.04307500    0.00122796    0.09597506    0.19412835    0.48653552
          0.01723000   -0.00041972    0.00074113    0.01327209    0.02807134
Th F
         14.88566000    0.00505744   -0.02310422    0.03164750
          4.54647000   -0.10958007    0.29600542   -0.40825344
          2.33642000   -0.25071209    0.60485377   -0.36582280
          1.13768000   -0.37476685   -0.03998639    0.82344579
          0.48203500   -0.36493260   -0.42738177    0.18385704
          0.19281400   -0.20122901   -0.30157096   -0.64757063
          0.07712600   -0.05237249   -0.07493980   -0.23549329
          0.03085000   -0.00416468   -0.00641273   -0.02203874
Th G
          4.05140000   -0.39050416   -0.61954067
          2.62680000   -0.14497714   -0.12104339
          1.25337200   -0.43643468    0.06754934
          0.59804300   -0.22671258    0.57762149
          0.28535500   -0.11743458    0.18337172
          0.12540600   -0.01366788    0.10101326
          0.07000000   -0.00788183   -0.00473646
Th H
          3.35510100    0.60387854
          1.71754800    0.20048876
          0.82913500    0.40376963
          0.40026000    0.04311932
```

```
          0.19322300    0.05181809
          0.09327700   -0.00896431
end

ecp
Th nelec 60
Th UL
   1      3.698978298569e+02      4.016886253269e+01
   1      2.477655967328e+02     -7.584009176330e+01
   2      2.011047071613e+02      1.119125617920e+03
   2      1.496430016110e+02     -9.390212475238e+02
   2      4.640820345015e+01     -1.589114782933e+02
   2      3.321312110134e+01      5.434909097838e+01
   2      2.327924832097e+01     -1.036155449222e+02
   2      1.209743694899e+01     -2.148789486174e+01
   2      6.715425102872e+00     -4.623176391720e+00
   2      3.730670044854e+00     -4.213014368523e-01
   2      8.740604208345e-01     -3.534684399247e-03
   2      5.314586854465e-01      1.299722959600e-03
   2      3.179053680476e-01     -4.241195633460e-04
   2      6.633123162449e-02     -1.706567934152e-05
   2      1.903637830472e-02     -3.046471463440e-06
   2      7.574215761278e-03      5.037219380614e-07
Th S
   0      1.856149912515e+02      1.000000000000e+01
   1      7.269610545713e+01      1.665689924021e+03
   1      5.062045400423e+01     -3.162409396416e+03
   1      2.445651582576e+01      1.544845564349e+03
   2      4.506701004658e+01      1.668603567121e+04
   2      3.236396577225e+01     -2.283898909532e+04
   2      2.347349275167e+01      1.712297056991e+04
   2      1.700920816888e+01     -1.649301164389e+04
   2      1.226004990448e+01      1.112252061428e+04
   2      8.807471578861e+00     -5.533354025347e+03
   2      6.303487518002e+00      2.410702817837e+03
   2      4.481012333236e+00     -9.512552942569e+02
   2      3.153715771217e+00      3.428842981648e+02
   2      2.192760596054e+00     -1.125329043970e+02
   2      1.503349725544e+00      3.274766569385e+01
   2      1.015838734318e+00     -8.158457770476e+00
   2      6.773386777800e-01      1.638261011147e+00
   2      4.466685408353e-01     -2.396255447742e-01
   2      2.906293427700e-01      1.796864033091e-02
Th P
   0      3.362238419942e+01      9.000000000000e+00
   1      1.086498486023e+02     -1.046019428867e+01
   1      6.344250624455e+01      3.208300662044e+01
   1      3.752508190866e+01      5.096372440818e+01
   1      2.382350781479e+01     -1.457224290972e+02
   1      1.422396131156e+01      1.195147818146e+02
   2      1.724977873564e+01      1.296825444132e+03
   2      1.219266888097e+01     -2.669812590136e+03
   2      8.799452270859e+00      2.764041714910e+03
   2      6.404530227360e+00     -1.592803841629e+03
   2      4.597933752868e+00      6.555382878557e+02
   2      3.234766507525e+00     -2.093159924852e+02
   2      2.230603879291e+00      5.228808778783e+01
   2      1.487030742906e+00     -8.966073167811e+00
```

```
   2      7.071096553715e-01      8.286892608804e-01
   2      3.868823593052e-01     -2.886767134097e-01
   2      2.269164855315e-01      1.169487079180e-01
   2      1.375627354920e-01     -3.939634409199e-02
   2      8.461830732000e-02      8.992871924271e-03
   2      5.210021826898e-02     -9.938193351190e-04
Th D
   0      4.706500063635e+01      7.000000000000e+00
   1      4.466520847650e+01      4.485949273483e+01
   2      2.141550252318e+01      2.838219406110e+02
   2      5.670309118951e+00      1.801522228446e+02
   2      4.051741257216e+00     -1.030854170907e+02
   2      2.643819122345e+00      3.190114097239e+01
   2      1.675404711619e+00     -9.788433414920e+00
   2      1.119651677234e+00      3.076109154373e+00
   2      7.541755684892e-01     -6.618044699546e-01
   2      5.018690850075e-01      7.279472517193e-02
Th F
   0      4.359501069915e+01      4.000000000000e+00
   1      2.748912440563e+01      4.855730389038e+01
   2      1.077953397751e+01      1.422668629080e+02
   2      2.098519361893e+00      1.793453855509e+01
   2      1.489976715733e+00     -1.559619347864e+01
   2      1.050385280915e+00      6.045555431934e+00
   2      7.271425950222e-01     -1.108492314274e+00
   2      4.904561671558e-01      7.302218497353e-02
end

so
Th P
   1      1.086498486023e+02      1.585953763839e+01
   1      6.344250624455e+01     -5.792827044666e+01
   1      3.752508190866e+01      1.884899442505e+02
   1      2.382350781479e+01     -2.963192187860e+02
   1      1.422396131156e+01      1.510903488594e+02
   2      1.724977873564e+01      7.345281508166e+02
   2      1.219266888097e+01     -1.107654283532e+03
   2      8.799452270859e+00      3.514271767696e+02
   2      6.404530227360e+00      1.784499233673e+02
   2      4.597933752868e+00     -2.145873572206e+02
   2      3.234766507525e+00      1.100750754714e+02
   2      2.230603879291e+00     -3.683701446161e+01
   2      1.487030742906e+00      7.645118981537e+00
   2      7.071096553715e-01     -8.526044933437e-01
   2      3.868823593052e-01      3.208157997071e-01
   2      2.269164855315e-01     -1.357477771601e-01
   2      1.375627354920e-01      4.743157917020e-02
   2      8.461830732000e-02     -1.127241359906e-02
   2      5.210021826898e-02      1.328462030120e-03
Th D
   1      4.466520847650e+01      1.764443189192e-01
   2      2.141550252318e+01      1.037029556088e+00
   2      5.670309118951e+00     -4.220102213462e+00
   2      4.051741257216e+00      7.631542413648e+00
   2      2.643819122345e+00     -3.546860648036e+00
   2      1.675404711619e+00      1.193250635161e+00
   2      1.119651677234e+00     -3.328202112641e-01
   2      7.541755684892e-01      5.233775775918e-02
```

```
   2      5.018690850075e-01     -2.997215417087e-03
Th F
   1      2.748912440563e+01      2.673136917106e-02
   2      1.077953397751e+01     -2.217784029274e-01
   2      2.098519361893e+00      1.504415595617e-01
   2      1.489976715733e+00      9.072108773711e-02
   2      1.050385280915e+00     -1.559605938103e-01
   2      7.271425950222e-01      6.089452880239e-02
   2      4.904561671558e-01     -7.683492875615e-03
Th G
   1      3.698978298569e+02     -2.918229100176e-01
   1      2.477655967328e+02      1.004286449808e+00
   2      2.011047071613e+02     -3.129165047537e+01
   2      1.496430016110e+02      3.485672969440e+01
   2      4.640820345015e+01     -2.422661483561e+00
   2      3.321312110134e+01      3.463214556493e+00
   2      2.327924832097e+01     -9.264683621459e-01
   2      1.209743694899e+01      9.917448844311e-02
   2      6.715425102872e+00     -1.776745284842e-02
   2      3.730670044854e+00      3.990511244671e-04
   2      8.740604208345e-01      6.862414542406e-04
   2      5.314586854465e-01     -1.838160561341e-04
   2      3.179053680476e-01      7.657922300082e-05
   2      6.633123162449e-02      3.421032844457e-06
   2      1.903637830472e-02     -1.273772767996e-07
   2      7.574215761278e-03      1.360326651964e-07
end
```
